# Supplementary material for: A learning scheme by sparse grids and Picard approximations for semilinear parabolic PDEs
Source: arXiv:2102.12051 source file (2021-02-24)
Supplement: Supplementary file 1 [file appendix.tex]

%!TEX root = main.tex
\section{Appendix}

\subsection{Proof of Lemma \ref{le space error any bounded domain}}
\label{subse app proof of lemma sparse grid error}
1. To $v:\R^d \rightarrow \R$, we associate $v_{|_{[\mathfrak{a},\mathfrak{b}]^d}}$ and
\begin{align*}
[0,1]^d \ni y \mapsto \tilde{v}(y) = v(\tau^{-1}(y)) \in \R\,,
\end{align*}
where 
\begin{align}
[\mathfrak{a},\mathfrak{b}]^d \ni x \mapsto \tau(x) = (\frac{x_1 - \mathfrak{a} }{\mathfrak{b} -\mathfrak{a}}, \dots, 
\frac{x_d - \mathfrak{a} }{\mathfrak{b}-\mathfrak{a}}
)^\top \in [0,1]^d\,.
\end{align}
We then compute, for $\mathbf{i}\in \mathbb{N}^d$
\begin{align}
\int_{[0,1]^d}|D^{\mathbf{i}}\tilde{v}(y)|^2 \ud y
&=\int_{[0,1]^d}
(\mathfrak{b}-\mathfrak{a})^{2|\mathbf{i}|_1} 
|D^{\mathbf{i}}v(\tau^{-1}(y))|^2\ud y \label{eq pour control sup}
\\
&= (\mathfrak{b}-\mathfrak{a})^{2|\mathbf{i}|_1-d} \int_{[\mathfrak{a},\mathfrak{b}]^d}
|D^{\mathbf{i}}v(x)|^2\ud x \label{eq pour control l2}
\end{align}
From \eqref{eq pour control sup}, we obtain
\begin{align}\label{eq control sup}
\int_{[0,1]^d}|D^{\mathbf{i}}\tilde{v}(y)|^2 \ud y
&\le 
(\mathfrak{b}-\mathfrak{a})^{2|\mathbf{i}|_1} |D^{\mathbf{i}}v|_\infty
\end{align}
and from \eqref{eq pour control l2}, we obtain
\begin{align} \label{eq control l2}
\int_{[0,1]^d}|D^{\mathbf{i}}\tilde{v}(y)|^2 \ud y
&\le 
 (\mathfrak{b}-\mathfrak{a})^{2|\mathbf{i}|_1-d} |D^{\mathbf{i}}v|_{L^2(\R^d)}
\end{align}
2. 
%\begin{align*}
%\inf_{w \in \mathscr{V}_n} \|w-v_{|_{\cO_n}}\|^2_{L^2(\cO_n)} 
%\end{align*}
Let us first observe that, for $w \in \mathscr{V}_n$
\begin{align}
\|w-v_{|_{\cO_n}}\|^2_{L^2(\cO_n)} & =
\int_{[\mathfrak{a}_n,\mathfrak{b}_n]^d}
|w(x)-v(x)|^2 \ud x
\\
&=(\mathfrak{b}_n-\mathfrak{a}_n)^{d}\int_{[0,1]^d}
|\tilde{w}(y)-\tilde{v}(y)|^2 \ud y
\end{align}
and we observe $\tilde{w} \in \mathscr{S}_{\ell_n}$. Since $w \mapsto \tilde{w}$ is one-to-one, we deduce
\begin{align*}
\inf_{w \in \mathscr{V}_n} \|w-v_{|_{\cO_n}}\|^2_{L^2(\cO_n)} 
&\le
(\mathfrak{b}_n-\mathfrak{a}_n)^{d}
\inf_{\tilde{w} \in \mathscr{S}_{\ell_n}} \| \tilde{w}-\tilde{v}\|_{L^2([0,1]^d)}
\\
&\le 
C_{d}(\mathfrak{b}_n-\mathfrak{a}_n)^{d} 2^{-4\ell_n} \ell_n^{d-1}\|\tilde{v}\|^2_{H^{2}_{mix}([0,1]^d)}
\end{align*}
where we used, for the last inequality above, \eqref{eq control sparse basic}.
\\
We then have
%\begin{align*}
%\|\tilde{v}\|^2_{H^{2}_{mix}([0,1]^d)} &\le C
%\sum_{\mathbf{j}\in \mathbb{N}^d, |\mathbf{j}|_\infty \le 2} |D^\mathbf{j}\tilde{v}|_2^2
%\\
%&\le C \sum_{\mathbf{j}\in \mathbb{N}^d, |\mathbf{j}|_\infty \le 2} 
%(\mathfrak{b}_n-\mathfrak{a}_n)^{2|\mathbf{j}|_1} |D^{\mathbf{j}}v|_\infty
%\end{align*}
%where we used \eqref{eq control sup} 
\begin{align*}
&\|\tilde{v}\|^2_{H^{2}_{mix}([0,1]^d)} \le C
\sum_{\mathbf{j}\in \mathbb{N}^d, |\mathbf{j}|_\infty \le 2} |D^\mathbf{j}\tilde{v}|_2^2
\\
&\le C \sum_{\mathbf{j}\in \mathbb{N}^d, |\mathbf{j}|_\infty \le 2, 2|\mathbf{j}|_1 \le d} 
(\mathfrak{b}_n-\mathfrak{a}_n)^{2|\mathbf{j}|_1} |D^{\mathbf{j}}v|_\infty
+
\sum_{\mathbf{j}\in \mathbb{N}^d, |\mathbf{j}|_\infty \le 2, 2|\mathbf{j}|_1 > d} 
(\mathfrak{b}_n-\mathfrak{a}_n)^{2|\mathbf{j}|_1-d} |D^{\mathbf{j}}v|_{L^2(\R^d)}
\end{align*}
where we used \eqref{eq control sup} and \eqref{eq control l2}. \eproof
%\textcolor{red}{to do}
%Go to the phd thesis of Bastian Bohn, definition 3.15 p21 states the norm equivalence between
%$H^2_{mix}$ and $W^2_{mix}$ and for this one we can compute the estimate by a change of variable. It is important to have the correct dependence upon $a$ in the bound given in Lemma \ref{le space error any bounded domain}.
